# Supplementary material for: Keep it Simple: Image Statistics Matching for Domain Adaptation
Source: arXiv:2005.12551 source file (2020-05-26)
Supplement: Supplementary file 1 [file appendix.tex]

or an additional section in the paper after results - limiting factors in the available public benchmarks:

\begin{itemize}
  \item Different labeling strategies between source and target domains (e.g. occluded objects - images with labels from various datasets)
  \item inaccurate bounding boxes in the GTA domain for occluded and far objects due to some limitations in the software used for the label extraction - refer to Roberson's paper
  \item Inconsistent categories between source and target domains (cars as vans or trucks) - it affects the evaluation
  \item Cityscapes: bounding boxes are unavailable in the far range (some ground truth boxes are incorrect in the ETH and Boston experiments)
  \item not sufficient amount of validation data in the Cityscapes domain (high variances in the mAP)
  \item different distributions of bounding box centroids in the data sets (KITTI, City, GTA)
  \item Fixed random seeds makes no sense and benefit (CACE principle: Changing Anything Changes Everything \cite{sculley2015hidden})
  \item Only one year season in KITTI and GTA (multiple in Cityscapes), night images exist only in the GTA
\end{itemize}
